# Supplementary material for: Phase-stable self-modulation of an electron-beam in a magnetic wiggler
Source: arXiv:1909.02166 source file (2019-09-05)
Supplement: Supplementary file 3 [file old_appendix.tex]

\iffalse

\section{Appendix}
In this appendix we discuss all of the approximations required to arrive at a simple expression for the electric field . Much of this section follows previous work~\cite{Geloni2005,kim2017,hofmann2007,wiedemann2007}, though experimental constraints allow us to apply some simplifications. The most comprehensive study~\cite{GELONI2007} of CSR in a wiggler is limited to wavelengths much greater than the resonant wavelength of the wiggler. Our goal in this section is to give an estimate for the modulation amplitude in the core of a beam with a current spike on the tail. We apply the following assumptions in this appendix
\begin{align}
    \text{no longitudinal field}\\
    \lambda_3 \ll \sigma_z \ll \lambda_1\\
    \boldsymbol{\phi} < a_u / \lambda_u
\end{align}

The inhomogeneous electromagnetic wave equation for the field $\mathbf{E}(x,y,z,t)$ from a source density $\rho$ and current density $\mathbf{J}$ is 
\begin{equation}
    \frac{1}{c^2}\frac{\partial^2 \mathbf{E}}{\partial t^2} -\nabla^2 \mathbf{E} = - \left( \frac{1}{\epsilon_0} \nabla \rho + \mu_0 \frac{\partial \mathbf{J}}{\partial t} \right).
    \label{maxwav}
\end{equation}
It is convenient to work in the frequency domain, defined by
\begin{align}
    f(t) &= \frac{1}{2\pi}\int d\omega e^{-i \omega t}\bar{f}(\omega)\\
    \bar{f}(\omega) &= \int dt e^{i \omega t} f(t).
\end{align}
With this transformation and the definition $k=\omega/c$, Equation~\ref{maxwav} becomes 
\begin{equation}
    \left(k^2 + \nabla^2\right) \bar{\mathbf{E}} = \frac{1}{2\pi \epsilon_0 c^2} \int dt e^{i \omega t} \left( \frac{\partial \mathbf{J}}{\partial t} + c^2 \nabla \rho \right).
    \label{wavfreq}
\end{equation}
We can express $\bar{\mathbf{E}}$ in terms of an envelope function $\Tilde{\mathbf{E}}$,
\begin{equation}
    \bar{\mathbf{E}} = \Tilde{\mathbf{E}} \, e^{ikz}. 
    \label{svea}
\end{equation}
Typically $\Tilde{\mathbf{E}}$ varies slowly over the length $\lambda=2\pi/k$ in the region of interest. We are most interested the field one wiggler period away from the source, a distance much larger than the resonant wavelength of the wiggler. Inserting Equation~\ref{svea} into  Equation~\ref{wavfreq} and applying the slowly varying envelope approximation to eliminate $\partial^2 \tilde{\mathbf{E}}/\partial z^2$, we arrive at 
\begin{equation}
    \left(2 i k \frac{\partial }{\partial z} + \nabla^2_{\!\! \perp}\right) \tilde{\mathbf{E}} = \frac{1}{2\pi \epsilon_0 c^2} \int dt e^{i (\omega t-kz)} \left( \frac{\partial \mathbf{J}}{\partial t} + c^2 \nabla \rho \right).
    \label{wavfreq2}
\end{equation}
At this point we neglect the longitudinal field, $E_z$. It can be show that this component vanishes in the far-field when $1/\gamma^2 \ll 1$~\cite{hofmann2007,wiedemann2007,Geloni2005}. This assumption has the effect of removing near-field effects such as longitudinal space charge. We therefore do not expect our analysis to be valid on the current spike. The transverse field is governed by
\begin{equation}
    \left(2 i k \frac{\partial }{\partial z} + \nabla^2_{\!\! \perp}\right) \tilde{\mathbf{E}}_{\perp} = \frac{1}{2\pi \epsilon_0 c^2} \int dt e^{i (\omega t-kz)} \left( \frac{\partial \mathbf{J}_{\! \perp}}{\partial t} + c^2 \nabla_{\! \! \perp} \rho \right).
    \label{wavfreq3}
\end{equation}
The transverse field is more easily handled in the angular domain,
\begin{align}
    \tilde{\mathbf{E}}_{\perp}(\mathbf{x}; z) &= \int d\boldsymbol{\phi} \, e^{i k \boldsymbol{\phi} \cdot \mathbf{x}} \tilde{\boldsymbol{\mathcal{E}}}(\boldsymbol{\phi};z),\\
    \tilde{\boldsymbol{\mathcal{E}}}(\boldsymbol{\phi};z) &= \frac{k^2}{(2\pi)^2} \int d\boldsymbol{x}  \, e^{-i k \boldsymbol{\phi} \cdot \mathbf{x}} \tilde{\mathbf{E}}_{\perp}(\mathbf{x}; z).
\end{align}
These transformations are applicable in the far-field, where the angle $\boldsymbol{\phi}$ between the propagation axis and the vector pointing from the source point to the observer is constant. The angular form of Equation~\ref{wavfreq3} is
\begin{equation}
    \left(\frac{\partial }{\partial z} +\frac{ik}{2} \boldsymbol{\phi}^2\right) \tilde{\boldsymbol{\mathcal{E}}} = -\frac{1}{4\pi \epsilon_0 c \lambda^2} \int dt d\boldsymbol{x} e^{i k (c t-z-\boldsymbol{\phi}\cdot \mathbf{x})} \left( \mathbf{J}_{\! \perp} - c \boldsymbol{\phi} \rho \right),
    \label{wavfreq4}
\end{equation}
where we have integrated by parts.

The source terms $\mathbf{J}_{\! \perp}$ and $\rho$ are most conveniently analyzed from a single electron perspective and generalized to a distribution through convolution. The source density and current density for a single electron are
\begin{align}
    \rho(\mathbf{r},t) &= -e \, \delta^3 (\mathbf{r} - \mathbf{r}_e(t))\\
    \mathbf{J}(\mathbf{r},t) &= \dot{\mathbf{r}}_e(t)\,\rho(\mathbf{r},t),
\end{align}
where the trajectory $\mathbf{r}_e$ and velocity $\dot{\mathbf{r}}_e = d\mathbf{r}_e/dt$ will be specified shortly. We will work under the assumption that the electron trajectories are determined a priori from the wiggler magnetic field alone, and that radiative effects can be ignored as far as the trajectory is concerned. In a wiggler, the electron speed, $v = |\mathbf{v}|$, is constant. It therefore traverses a distance $s(z) = v \, t(z)$ after some time $t(z)$. This fact allows the longitudinal and time dependence of $\rho$ to be interchanged,
\begin{align}
    \rho(\mathbf{r},t) &= -e \delta (x-x_e(t))\delta (y-y_e(t))\delta (z-z_e(t))\\
    &= -e \delta (x-x_e(z))\delta (y-y_e(z)) \frac{\delta\left(\frac{s(z)}{v} - t\right)}{\dot{z}(z)}.
\end{align}
In a wiggler of strength $K$ and magnetic polarization in along the y-axis, relevant components of the electron trajectory expanded through $O(1/\gamma^2)$ are~\cite{kim2017}
\begin{align}
    x_e(z) &\approx \frac{K}{\gamma k_u} \sin (k_u z)\\
    y_e(z) &=0\\
    c\frac{s(z)}{v} &\approx \left(1+\frac{1+K^2/2}{2\gamma^2}\right)z + \frac{K^2}{8\gamma^2 k_u}\sin(2 k_u z)\\
    \dot{x}_e(z)/c &\approx \frac{K}{\gamma}\cos (k_u z)\\
    \dot{y}_e(z)/c &= 0\\
    \dot{z}_e(z)/c &\approx 1-\frac{1+K^2/2}{2\gamma^2} - \frac{K^2}{4\gamma^2} \cos (2 k_u z).
\end{align}
Inserting these into Equation~\ref{wavfreq4} we find 
\begin{equation}
    \left(\frac{\partial }{\partial z} +\frac{ik}{2} \boldsymbol{\phi}^2\right) \tilde{\boldsymbol{\mathcal{E}}} = 
    \frac{e (\boldsymbol{\beta}_{\! \perp}(z) - \boldsymbol{\phi})}{4\pi \epsilon_0 \lambda^2 \dot{z}_e} e^{i k (c s/v-z-\boldsymbol{\phi}\cdot \mathbf{x})}.
    \label{wavfreq5}
\end{equation}
If we assume our wiggler begins at $z=0$, the solution to Equation~\ref{wavfreq5} is
\begin{align}
    \tilde{\boldsymbol{\mathcal{E}}} =& \int_0^z dz' \frac{e(\boldsymbol{\beta}_{\! \perp}(z') - \boldsymbol{\phi})}{4\pi\epsilon_0\lambda^2 c} e^{i \psi(z')},\label{intphase}\\
    \psi(z') 
    =& \, k \left(\frac{c s(z')}{v}-z'-\boldsymbol{\phi}\cdot \mathbf{x}(z') + \boldsymbol{\phi}^2 \frac{z'-z}{2}\right) \nonumber\\
    =& \, k \, \bigg(\frac{1+K^2/2}{2\gamma^2}z' + \frac{K^2}{8k_u \gamma^2}\sin(2 k_u z') \nonumber\\
    & \, -\frac{K}{\gamma k_u}\phi_x \sin(k_u z') + \boldsymbol{\phi}^2 \frac{z'-z}{2}\bigg),
    \label{toint}
\end{align}
where $\boldsymbol{\beta}_{\! \perp}(z') - \boldsymbol{\phi} = ((K/\gamma) \cos (k_u z') -\phi_x)\hat{x} - \phi_y \hat{y}$, and the $\dot{z}_e$ in the denominator of Equation~\ref{wavfreq5} was replaced with $c$ and the oscillation amplitude $a_u = K/\gamma k_u$ was used. This integral can be evaluated and expanded into harmonics via two applications of the Jacobi-Anger identity. The integrand becomes
\begin{align}
    &(\boldsymbol{\beta}_{\! \perp}(z') - \boldsymbol{\phi}) e^{i \psi(z')} =\nonumber\\ &\,\,\,\,\,\,\, \left[\frac{K}{2\gamma} \left(e^{ik_u z'}+e^{-ik_u z'}\right) -\phi_x, - \phi_y\right]\nonumber\\ 
    &\,\, \times \sum_{n=-\infty}^\infty \sum_{m=-\infty}^\infty J_n\left(\frac{k K^2}{8 k_u \gamma^2}\right) J_m\left(-\frac{k K}{k_u \gamma}\phi_x\right)\nonumber\\
    &\,\, \times \exp\bigg( i k_u z' \bigg( \frac{k}{k_1} + 2n+m    \bigg) +
    i k \boldsymbol{\phi}^2\frac{z'-z}{2}\bigg),
    \label{wholeshebang}
\end{align}
where 
\begin{equation}
    k_1 = k_u \frac{2 \gamma^2}{1+K^2/2}.
\end{equation}
We are now in position to calculate the total power emitted by the source. Equation \ref{toint} can be evaluated with the integrand given in Equation~\ref{wholeshebang}. We
\begin{equation}
    a
\end{equation}

Our goal in this Appendix is to describe the radiation from the beam tail capable of modulating the beam core. This interaction only involves radiation forming at angles small enough to interact with the beam one or more wiggler wavelength away, $|\boldsymbol{\phi}| < a_u / \lambda_u = K/2\pi \gamma.$ This is a factor of $2\pi$ smaller than the transverse velocity $|\boldsymbol{\beta}_\perp| = K/\gamma$. We therefore ignore the angular dependence of $\boldsymbol{\beta}_{\! \perp}(z') - \boldsymbol{\phi}$. We do so with the knowledge that any calculation of the beam power will be incorrect if the region of angular coherence, $|\boldsymbol{\phi}| < \sqrt{2}/k \sigma$ for a Gaussian electron beam, is larger than $K/\gamma$. The unsatisfied reader can refer to other references~\cite{hofmann2007} for a calculation of the far-field power from a wiggler. With this simplification the integrand becomes 
\begin{align}
    &\beta_{x}(z') e^{i \psi(z')} =\frac{K}{2\gamma} \sum_{n,m} J_n\left(\frac{k K^2}{8 k_u \gamma^2}\right) J_m\left(-\frac{k K}{k_u \gamma}\phi_x\right)\nonumber\\
    &\,\, \times \exp\bigg( i k_u z' \bigg( \frac{k}{k_1} + 2n+m  \pm 1  \bigg) +
    i k \boldsymbol{\phi}^2\frac{z'-z}{2}\bigg),
    \label{wholeshebang2}
\end{align}
where the $\pm$ represents the two terms arising from the complex representation of $\cos k_u z'$. Inserting Equation~\ref{wholeshebang2} into Equation~\ref{intphase} and integrating gives 
\begin{align}
    \tilde{\boldsymbol{\mathcal{E}}} &=\frac{Kz}{8\pi \epsilon_0 \lambda^2 c \gamma} \sum_{m,n} J_n\left(\frac{k K^2}{8 k_u \gamma^2}\right) J_m\left(-\frac{k K}{k_u \gamma}\phi_x\right)\nonumber \\
    &\,\,\,\,\,\,\, \times \exp \left( i\frac{z k_u}{2} \left(\frac{k}{k_1} +2n + m\pm 1  +  \frac{k}{2k_u} \boldsymbol{\phi}^2 \right)\right)\nonumber\\
    &\,\,\,\,\,\,\, \times \text{sinc} \left( \frac{z k_u}{2}\left(\frac{k}{k_1} +2n + m\pm 1  +  \frac{k}{2k_u} \boldsymbol{\phi}^2 \right) \right)
\end{align}


To further simplify this expression, we note that the longitudinal extent of the current spike restricts coherent emission to frequencies around or below $k_1$. This restriction, combined with the 

The angular restriction $|\boldsymbol{\phi}| < a_u / \lambda_u$ also restricts 

The dominant contribution to the integral in Equation~\ref{intphase} comes from frequencies $k$ resulting in a stationary phase. The phase, which .  The $\cos (k_u z)$ from $\boldsymbol{\beta}_\perp$ can also be inserted into 

%In this work we assume the unit vector pointing from the source to the observer is independent of time. This approximation is common in the literature~\cite{hofmann2007}, and it results in the removal of the velocity term in the Li\'enard--Wiechert expression for the field from a moving charge~\cite{Geloni2005}. 


\fi
